# Supplementary material for: Shape-Space Deformer: Unified Visuo-Tactile Representations for Robotic Manipulation of Deformable Objects
Source: arXiv:2409.12419 source file (2025-05-18)
Supplement: Supplementary file 1 [file supplementary.tex]

\section{Appendix}

    \begin{figure}[H]
        \centering
        \includegraphics[width=1\linewidth]{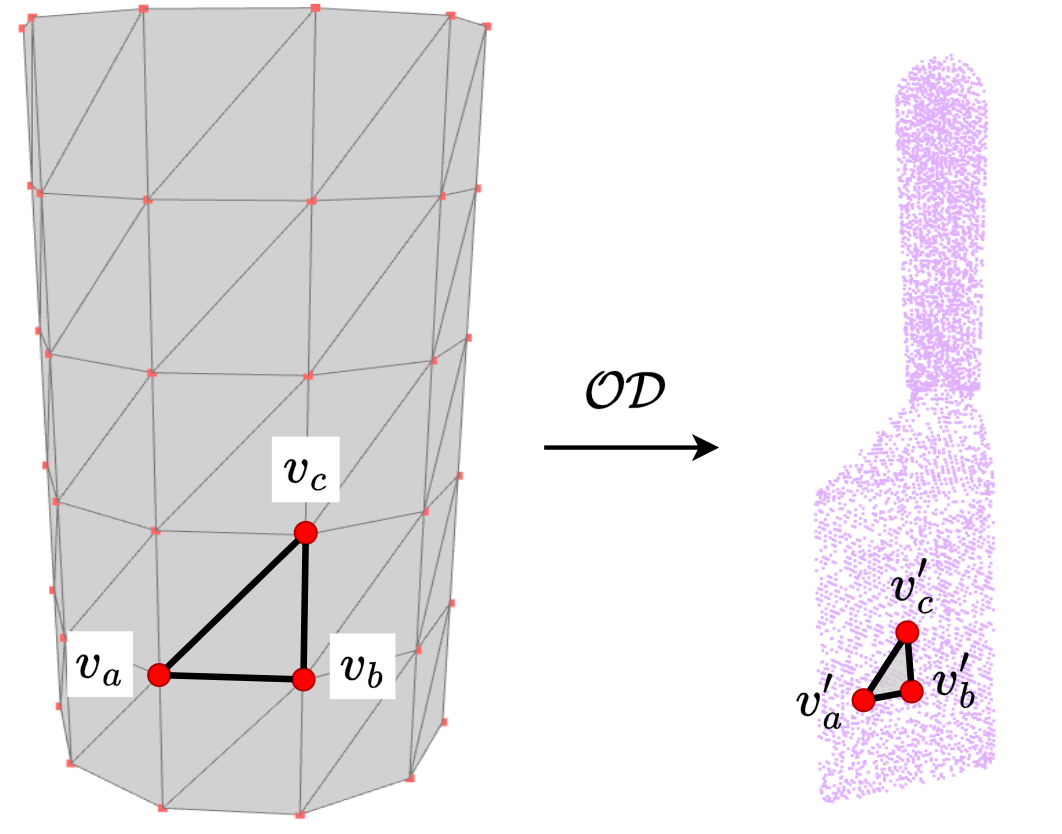}
        \caption{Deforming a template mesh means that vertex connections, and thus a mesh representation, are maintained.}
        \label{fig:triangles}
    \end{figure}

    \begin{figure}[H]
        \centering
        \includegraphics[width=1\linewidth]{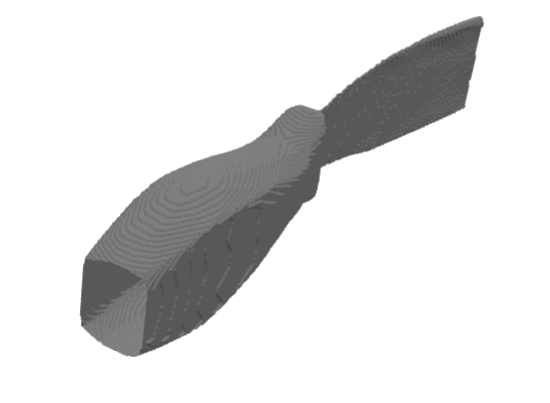}
        \caption{
        Hole present in mesh reconstruction of Shape 0, created by rendering the SDF model from \cite{Youngsun_2022_VIRDO}.
        % As a result of scaling coordinates to be $\pm{1}$, 
        In each shape there are not enough sample points given at the top of the handle to distinguish the boundary, thus leaving an open hole in rendering.
        }
        \label{fig:shape0_open_hole}
    \end{figure}

    % \begin{figure}[t!]
    %     \centering
    %     \includegraphics[width=1\linewidth]{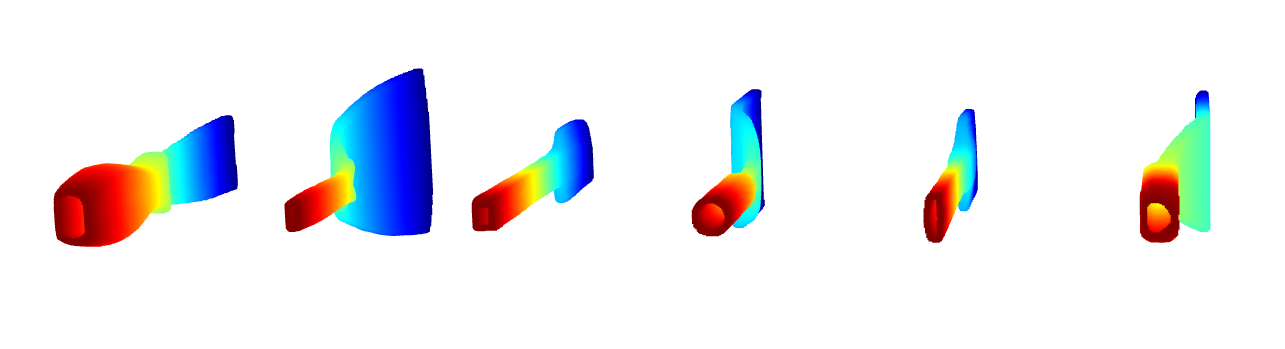}
    %     \caption{
    %         As a result of scaling coordinates to be $\pm{1}$, 
    %     }
    %     \label{fig:object_sdf_holes}
    % \end{figure}

    \begin{figure}[H]
        \centering
        \includegraphics[width=1\linewidth]{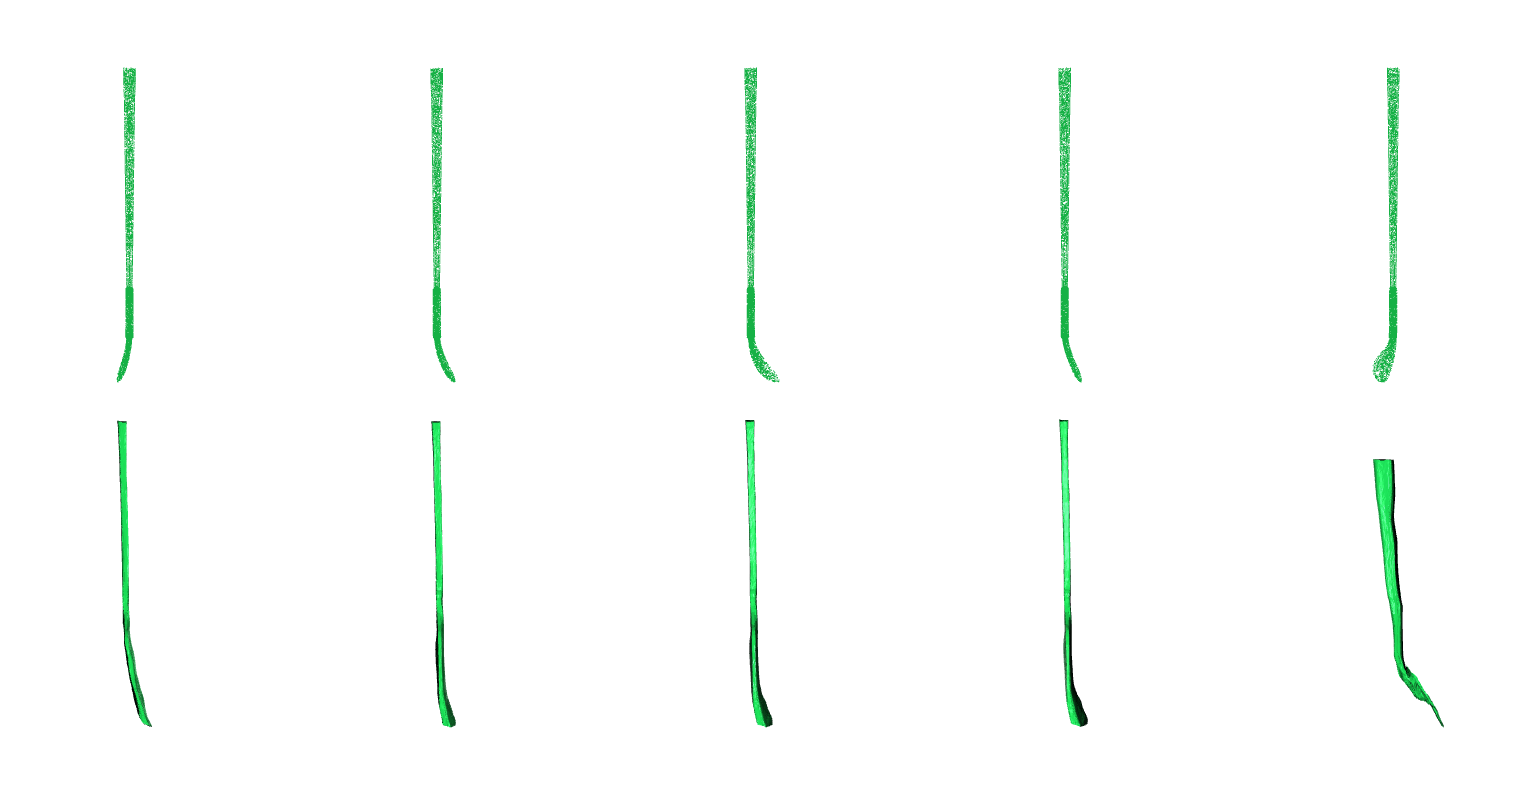}
        \caption{
            First row: Ground truth.
            Second row: Test-time reconstructions on five shapes from the \ExperimentEight{} experiment.}
        \label{fig:one_object_blindform_results}
    \end{figure}

    % \begin{figure}[H]
    %     \centering
    %     \includegraphics[width=1\linewidth]{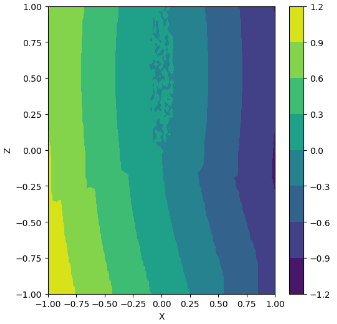}
    %     \caption{Enter Caption}
    %     \label{fig:enter-label}
    % \end{figure}

    \begin{figure}[H]
        \centering
        \includegraphics[width=1\linewidth]{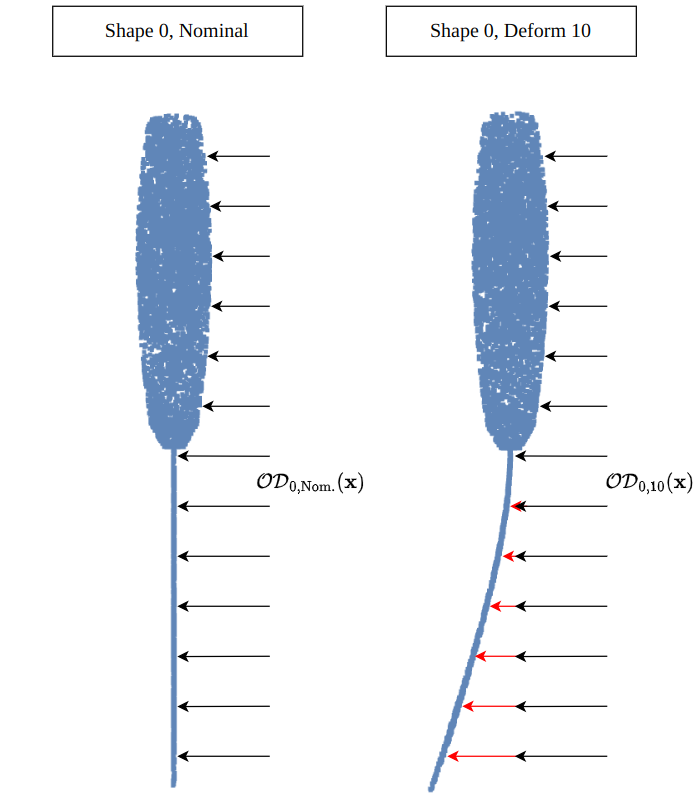}
        \caption{The surface deformation field for nominal and deformed shapes share a great deal of similarity }
        \label{fig:nom_vs_def_field}
    \end{figure}

    \begin{figure}[H]
        \centering
        \includegraphics[width=0.5\linewidth]{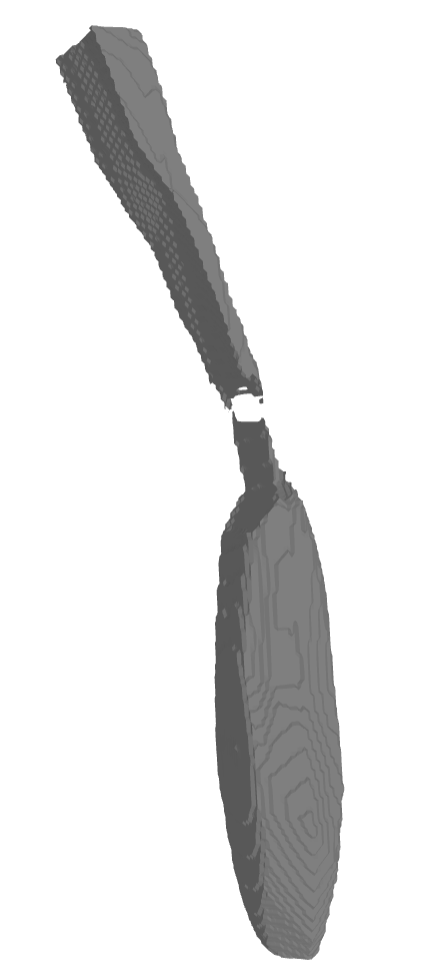}
        \caption{Shape 0, deform 12, \ExperimentThree, VIRDO }
        \label{fig:enter-label}
    \end{figure}
    
    \begin{figure}[H]
        \centering
        \includegraphics[width=0.6\linewidth]{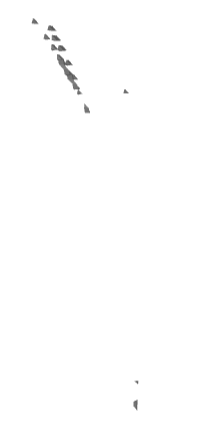}
        \caption{Shape 3, deform 73, \ExperimentThree, VIRDO }
        \label{fig:enter-label}
    \end{figure}
